# Supplementary material for: From Research Goals to Scientific Closure: Evaluating Agents Through Evidence-Supported Physics Research
Source: arXiv:2610.21767 source file (2026-10-15)
Supplement: Supplementary file 1 [file grading_prompt_style.tex]

% Shared palette with Appendix A.3; separate names avoid changing its casebox.
\RequirePackage{xcolor}
\RequirePackage[skins,breakable]{tcolorbox}
\RequirePackage{ragged2e}
\definecolor{gradingtemplateblue}{RGB}{40,78,116}
\definecolor{gradingmintblue}{RGB}{224,240,245}
\definecolor{gradingmintframe}{RGB}{161,185,199}
\definecolor{gradingminttitle}{RGB}{56,100,125}
\newtcolorbox{gradingprompt}[1]{
    enhanced,
    breakable,
    skin first=enhanced,
    skin middle=enhanced,
    skin last=enhanced,
    colback=gradingmintblue!40!white,
    colframe=gradingmintframe,
    colbacktitle=gradingminttitle!15!white,
    coltitle=gradingtemplateblue,
    title=\textbf{#1},
    title after break=\textbf{#1 (continued)},
    fonttitle=\bfseries,
    fontupper=\normalsize,
    sharp corners=south,
    boxrule=0.8pt,
    arc=6pt,
    left=6pt, right=6pt, top=6pt, bottom=6pt,
    before upper={\RaggedRight\setlength{\parskip}{3pt}},
    before skip=6pt, after skip=6pt
}
